# Supplementary material for: CompoSE: Compositional Synthesis and Editing of 3D Shapes via Part-Aware Control
Source: arXiv:2605.19350 source file (2026-10-03)
Supplement: Supplementary file 1 [file supp-acmtog.tex]

\documentclass[acmtog,nonacm]{acmart}
\setcopyright{acmlicensed}
\copyrightyear{2026}
\acmYear{2026}
\acmDOI{XXXXXXX.XXXXXXX}
\acmJournal{TOG}
\acmVolume{1}
\acmNumber{1}
\acmArticle{1}
\acmMonth{1}
\acmSubmissionID{1855}
\citestyle{acmauthoryear}

\input{preamble}

\usepackage[most]{tcolorbox}
\usepackage{xcolor}
\definecolor{promptbordercolor}{RGB}{30, 90, 160}
\definecolor{promptbgcolor}{RGB}{245, 248, 253}
\definecolor{prompttitlecolor}{RGB}{30, 90, 160}
 
\newtcolorbox{promptbox}[1][]{%
  enhanced,
  breakable,
  colback=promptbgcolor,
  colframe=promptbordercolor,
  colbacktitle=prompttitlecolor,
  coltitle=white,
  fonttitle=\bfseries\sffamily,
  title=#1,
  boxrule=0.8pt,
  arc=3pt,
  left=8pt,
  right=8pt,
  top=10pt,
  bottom=10pt,
  attach boxed title to top left={yshift=-2mm, xshift=4mm},
  boxed title style={
    colframe=promptbordercolor,
    boxrule=0.6pt,
    arc=2pt,
  },
}

\begin{document}

\title{CompoSE: Compositional Synthesis and Editing of 3D Shapes via Part-Aware Control}

\vspace{1em}

\input{sec/X_suppl}

\newpage
\bibliographystyle{ACM-Reference-Format}
\bibliography{citations}

\end{document}
